# Supplementary material for: Indirect measurement of the carbon adatom migration barrier on graphene
Source: arXiv:2202.04485 source file (2022-02-09)
Supplement: Supplementary file 1 [file supplemental_material_text.pdf]

# SUPPLEMENTAL MATERIAL

# Indirect measurement of the carbon adatom migration barrier on graphene

Andreas Postl,* Pit Pascal Patrick Hilgert, Alexander Markevich,
Jacob Madsen, Kimmo Mustonen, Jani Kotakoski, and Toma Susi†
*University of Vienna, Faculty of Physics,*
*Boltzmanngasse 5, A-1090 Vienna, Austria.*

(Dated: February 5, 2022)

**CONTENTS**


A. Knock-on damage cross section 3
  1. Experimental 3
  2. Theoretical 4
B. Arrhenius formalism for estimation of the adatom migration energy barrier 7
C. Extended model for competing knock-on damage and vacancy healing 9
  1. Discussion 9
  2. Formalism 10
  3. Adatom concentration and temperature-dependence 13
D. Probe-shape measurement 14
E. Experimental data 15
  1. Measured knock-on damage cross sections 15
  2. Beam-current calibration 15
F. Uncertainty estimation 18
  1. Beam current 18
  2. Electron count 18
  3. Experimental cross section 19
  4. Observed knock-on rate 19
  5. Theoretical cross section 19
  6. Predicted knock-on rate 20
  7. Migration energy barrier (Arrhenius formalism) 20

References 21



* andreas.postl@univie.ac.at

† toma.susi@univie.ac.at

### A. Knock-on damage cross section

#### 1. Experimental

The total number of electrons $N_{e^-}$ until the first defect was observed was calculated from image metadata based on beam current measurements (see section E 2 below). For the defect frame, we counted half of the full frame time and neglected the $(x, y)$ position of the defect:

$$N_{e^-} = \frac{1}{e}\left(\left(\sum_{j=1}^{\star-1} t_j I_{B,j}\right) + \frac{t_\star}{2} I_{B,\star}\right), \tag{1}$$

where $e$ is the elementary charge, $t_j$ is the time span between the end of the $(j+1)$-th and the end of the $j$-th frame, $I_{B,j}$ is the corresponding beam current during the acquisition of the $j$-th frame, and the sign '$\star$' labels the defect frame.

For a homogeneous Poisson process, the expected number of electrons per knock-on event is time-independent and, thus, not a function of the beam current. It is exponentially distributed with expectation value $\lambda$ and the density function

$$p_\lambda\left(N_{e^-}\right) = \begin{cases} \frac{1}{\lambda} e^{-\frac{N_{e^-}}{\lambda}} & \text{for } N_{e^-} \geq 0 \\ 0 & \text{for } N_{e^-} < 0 \end{cases}. \tag{2}$$

$\lambda$ is obtained from the experimental data by analyzing the measured doses per displacement as resulting from a Poisson process, as described below. The expectation value for the cross section for knock-on damage is then given by

$$\sigma = \frac{1}{\rho_A}\frac{N_{ko}}{N_{e^-}} = \frac{1}{\rho_A \lambda} \quad \text{with} \quad \rho_A = 2\frac{1}{A_{UC}} = \frac{4}{a_{gra}^2\sqrt{3}}, \tag{3}$$

for areal atomic density $\rho_A$; $A_{UC}$ is the graphene unit cell area, $a_{gra}$ its lattice constant, and $N_{ko}$ the number of knock-on damage events and $N_{e^-}$ number of electrons. Although it would have been consistent to fit the probability density function (Eq. (2)) to a normalized histogram of our set of $M$ total electron counts $\left\{N_{e^-}^{(i)} \mid k = 1, 2, ..., M\right\}$, the method becomes more robust to outliers if we use the data points

$$y(x) := \sum_{i=1}^{M} \Theta\left(N_{e^-}^{(i)} \geq x\right), \tag{4}$$

where $\Theta$ is the Heavyside step function and $x$ denotes the histogram bin edges, and a non-normalized negative exponential function is fitted. This takes advantage of the relationship

$$y_\lambda(x) := \begin{cases} \int_x^\infty p_\lambda(N_{\mathrm{e}^-})\,\mathrm{d}N_{\mathrm{e}^-} = e^{-\frac{x}{\lambda}} & \text{for } x \geq 0 \\ 0 & \text{for } x < 0 \end{cases} . \tag{5}$$

Fitting $y_\lambda$ yields its estimation value with a statistical uncertainty $\Delta\lambda$ for the electron count until a knock-on event happened.

*2. Theoretical*

The relativistic energy-momentum conservation leads to an elastic energy transfer

$$\begin{aligned} E(E_e, v, \theta) &= \frac{1}{2Mc^2}\left[2\,(1-\cos\theta)\left(E_e\left(E_e + 2m_0c^2\right) + \sqrt{E_e\left(E_e + 2m_0c^2\right)Mvc}\right) + (Mvc)^2\right] \\ &\approx E_{\max}\left(E_e, v\right)\sin^2\left(\frac{\theta}{2}\right) \end{aligned} \tag{6}$$

from an impinging electron with mass $m_0$ and a kinetic energy $E_e$ to a nucleus with mass $M$ moving at a velocity $v$ parallel to the electron momentum, depending on the electron scattering angle $\theta$ [1]. $c$ is the speed of light in vacuum. Here, we introduced the maximum transferred energy $E_{\max}\left(E_e, v\right) := E\left(E_e, v, \theta = 2\pi\right)$ for back-scattering at an angle of 180°.

As derived by Seitz and Koehler [2] and recently discussed in depth (e.g. [1, 3, 4]), Mott scattering [5, 6] with the McKinley and Feshbach expansion [7] and the assumption of an isotropic displacement threshold energy $T_{\mathrm{d}}$ results in a displacement cross section for knock-on damage as a function of the electron's kinetic energy and the nucleus' velocity $v$ parallel to the electron momentum due to energy transfer $E_{\max}(E_e, v)$ as

$$\begin{aligned} \tilde{\sigma}_{\mathrm{ko}}(E_e, v) = 4\pi &\left(\frac{Ze^2}{8\pi\epsilon_0 m_0 c^2\gamma\beta^2}\right)^2 \\ &\left\{\frac{E_{\max}}{T_{\mathrm{d}}} - 1 - \beta^2\log\left(\frac{E_{\max}}{T_{\mathrm{d}}}\right) + \pi Z\alpha\beta\left[2\sqrt{\frac{E_{\max}}{T_{\mathrm{d}}}} - \log\left(\frac{E_{\max}}{T_{\mathrm{d}}}\right) - 2\right]\right\}, \end{aligned} \tag{7}$$

where $Z$ denotes the atomic number, $e$ the elementary charge, $\epsilon_0$ the vacuum permittivity, and $\alpha$ the fine structure constant. The relativistic factor and the Lorentz factor of the impinging electron are given respectively by $\beta(E_e) = \sqrt{1 - \left(1 + E_e/m_0/c^2\right)^{-2}}$ and $\gamma(E_e) = \left(1-\beta^2\right)^{-1/2}$.

To obtain the displacement cross section as a function of temperature, we estimate the root-mean-square velocity $v_{\mathrm{rms}}(T)$ (in Ref. [4] denoted as $\overline{v^2(T)}^{1/2}$), from the phonon density of states (DOS), giving the out-of-plane velocity distribution

$$p(v,T) = \frac{1}{v_{\mathrm{rms}}(T)\sqrt{2\pi}} \exp\left(-\frac{v^2}{2(v_{\mathrm{rms}}(T))^2}\right), \tag{8}$$

and integrate the product of equations (7) and (8) inside the velocity domain over which the knock-on condition $E_{\mathrm{max}}(E_e, v) > T_{\mathrm{d}}$ is satisfied [1, 4], giving the total knock-on cross section $\sigma_{\mathrm{ko}}$ as a function of the electron's kinetic energy and the temperature:

$$\sigma_{\mathrm{ko}}(E_e,T) = \int_{-\infty}^{\infty} \Theta\left(E_{\mathrm{max}}(E_e,v) - T_{\mathrm{d}}\right) p(v,T)\tilde{\sigma}_{\mathrm{ko}}(E_e,v)\, dv\,. \tag{9}$$

The limits for the numerical integration were chosen as $v_{\mathrm{min}} = 0$ (because here $\forall v \leq 0 :$ $E_{\mathrm{max}}(E_e, v) < T_{\mathrm{d}}$) and $v_{\mathrm{max}} = 8v_{\mathrm{rms}}(T)$, so that the velocity distribution is fully sampled.

Due to possible inaccuracies in our model [4], the displacement threshold energy $T_{\mathrm{d}}$ and out-of-plane root-mean-square velocity of the nuclei $v_{\mathrm{rms}}(T)$ were allowed to vary within reasonable limits. We performed a non-linear regression to fit the model to our voltage-dependent data at ambient temperature (see Fig. 1). The experimental cross section at 90 keV is now accurately measured to be (13.6 ± 0.5) mb, whereas the data for 85, 95 and 100 kV stem from earlier measurements with less statistics. Variance-weighted least squares with a trust region reflective algorithm [8] yielded $T_{\mathrm{d}} = (21.03 \pm 0.10)$ eV and a $v_{\mathrm{rms}}^{\mathrm{opt}}(T) = (1.05 \pm 0.03)v_{\mathrm{rms}}^{\mathrm{phDOS}}(T)$. Notably, this slightly higher velocity than theoretically predicted was required to accommodate both the newly measured 90 keV datapoint and the older data, and the corresponding fitted threshold energy is slightly lower than previously estimated.

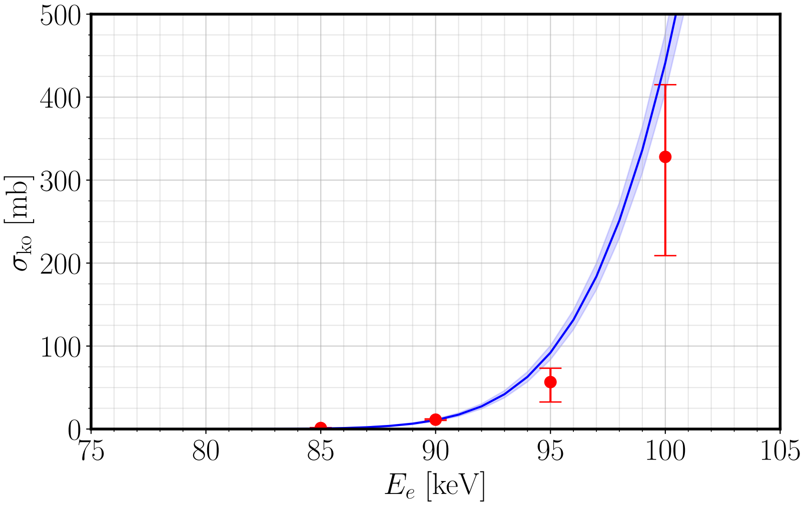


Supplemental Figure 1. Experimental (red points) and theoretically modeled (blue line) cross section for knock-on damage as a function of incident electron energy $E_e$ at $T = 300$ K.

### B. Arrhenius formalism for estimation of the adatom migration energy barrier

The Arrhenius equation describes the rate $k_{\mathrm{m}}$ (often referred to as rate constant) of the single-atom surface migration process as

$$k_{\mathrm{m}}(T) = A \exp\left(-\frac{E_{\mathrm{m}}}{k_{\mathrm{B}} T}\right), \tag{10}$$

where $A$ is the pre-exponential factor corresponding to a trial frequency, $E_{\mathrm{m}}$ the migration energy barrier, $k_{\mathrm{B}}$ the Boltzmann constant, and $T$ the absolute temperature.

To approximate the healing rate $k_{\mathrm{h}}$ of single vacancies in graphene by adatom diffusion and recombination, we postulate that the energy barrier $E_{\mathrm{r}}$ for the recombination of a carbon adatom in the immediate proximity of a single vacancy is negligible compared to the surface migration barrier, i.e.,

$$\begin{aligned} E_{\mathrm{r}} \ll E_{\mathrm{m}} \quad &\Rightarrow \quad k_{\mathrm{r}}(T) \gg k_{\mathrm{m}}(T), \\ \frac{1}{k_{\mathrm{h}}} = \frac{1}{k_{\mathrm{r}}} + \frac{1}{k_{\mathrm{m}}} \approx \frac{1}{k_{\mathrm{m}}} \quad &\Rightarrow \quad k_{\mathrm{h}}(T) \approx k_{\mathrm{m}}(T). \end{aligned} \tag{11}$$

Further, we compare the theoretically predicted knock-on damage rate $k_{\mathrm{ko}}^{\mathrm{theor}}(I_{\mathrm{B}}, T)$ to the experimentally observed knock-on rate $k_{\mathrm{ko}}^{\mathrm{obs}}(T)$, and assume that their difference is given by the healing rate,

$$k_{\mathrm{ko}}^{\mathrm{theor}}(I_{\mathrm{B}}, T) - k_{\mathrm{ko}}^{\mathrm{obs}}(T) \approx k_{\mathrm{h}}(T) \approx A \exp\left(-\frac{E_{\mathrm{m}}}{k_{\mathrm{B}} T}\right), \tag{12}$$

which allows us to obtain an estimate for the surface migration barrier via an Arrhenius fit of a line to the data points $\left(\frac{1}{T}, \log\left(k_{\mathrm{ko}}^{\mathrm{theor}} - k_{\mathrm{ko}}^{\mathrm{obs}}\right)\right)$, since taking the logarithm of equation (12) gives

$$\log\left(k_{\mathrm{ko}}^{\mathrm{theor}} - k_{\mathrm{ko}}^{\mathrm{obs}}\right) \approx \log A - \frac{E_{\mathrm{m}}}{k_{\mathrm{B}}} \frac{1}{T}. \tag{13}$$

The Arrhenius fit visualized in Suppl. Fig. 2 was performed using orthogonal distance regression [9], yielding $E_{\mathrm{m}} = (150 \pm 6)$ meV for the adatom migration barrier and $A = (2.1 \pm 0.2)\ \mathrm{s}^{-1}$ for the pre-exponential factor.

We note that the Arrhenius equation could be modified with a temperature-dependent pre-exponential factor ($A = BT^r, r \approx 1/2$) [10], but we decided to omit this as it would have a negligible effect on the present results.

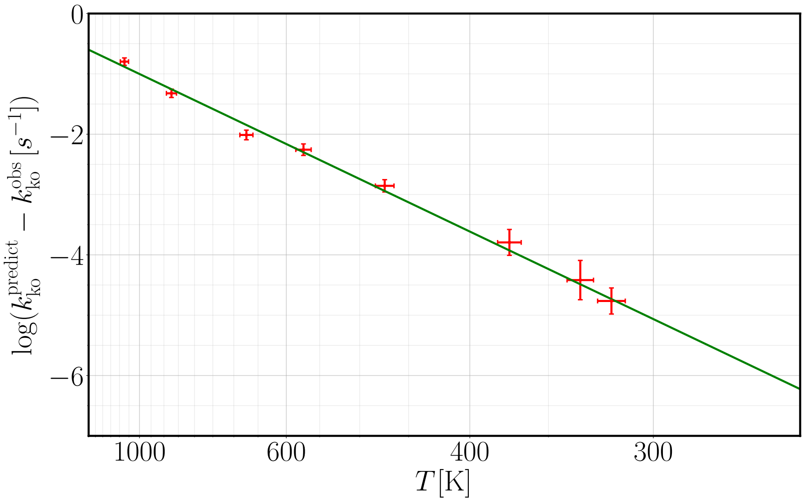


Supplemental Figure 2. Arrhenius plot of the defect healing rate with experimental estimates (red points) and a linear fit using orthogonal distance regression (green line).

### C. Extended model for competing knock-on damage and vacancy healing

#### 1. *Discussion*

As discussed in the main text, the naive Arrhenius fit described above is not an appropriate model for the experimental measurement, which is evident from the pre-exponential factor that is strictly limited to our frame time. To discuss the extended model that takes into account the finite scanning probe, let us first recap the behavior of knock-on damage and vacancy healing at elevated temperatures.

Limited by the experimental signal-to-noise ratio, we were able to lower the frame time down only to roughly half a second (although at fixed temperatures, there was no clear trend with respect to the frame time between 0.5 s and 2 s). However, the expected healing rate for elevated temperatures ($T \geq 500$ K) is orders of magnitude higher than the knock-on damage rate for beam currents in the range of 50–100 pA. The temperature-dependence of the expected knock-on damage cross section and the reaction rate of a generic physical or chemical process in which an energy barrier needs to be overcome are depicted in Suppl. Figs. 3 and 4. Only at very high temperatures does the relative slope of our theoretical cross section curve become higher than the relative slope of a generic reaction process rate.

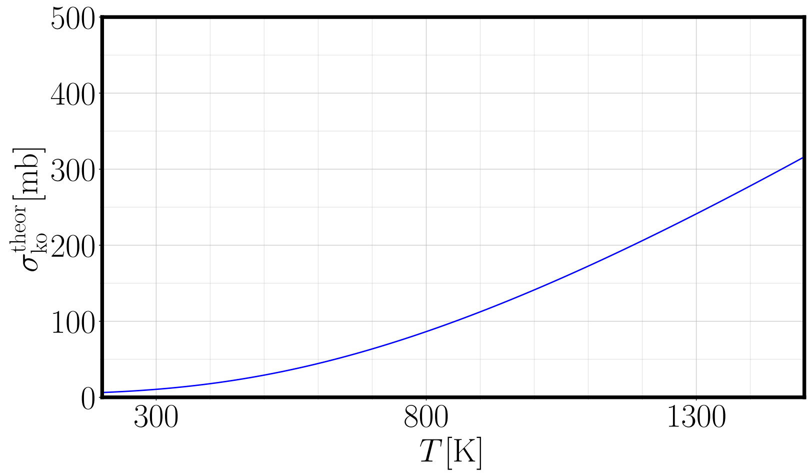


Supplemental Figure 3. Predicted knock-on damage cross section $\sigma^{\mathrm{theor}}(T)$ for 90 keV electrons as a function of temperature.

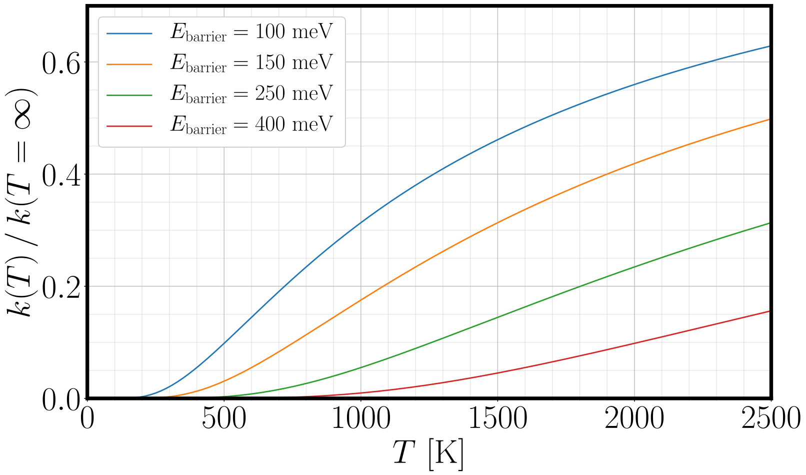


Supplemental Figure 4. Relative reaction process rate $k(T)/k(T=\infty)$ as a function of temperature for different (activation) energy barriers $E_{\mathrm{barrier}}$.

*2. Formalism*

To develop the extended model, we first treat adatom migration (in isolation, disregarding vacancy healing) as a Bernoulli process [11]. Thus, the number of migration steps for one adatom within one frame time $n_{\mathrm{f}}(T)$ obeys the binomial distribution

$$n_{\mathrm{f}}(T) \sim \mathcal{B}(n, p(T)) \tag{14}$$

with the distribution parameters

$$n = t_{\mathrm{f}} f_0, \quad p(T) = \exp\left(-\frac{E_{\mathrm{m}}}{k_{\mathrm{B}}T}\right), \tag{15}$$

where $t_{\mathrm{f}}$ denotes the frame time, and $f_0$ the trial frequency or attempt rate. Typical values are $t_{\mathrm{f}} = 0.5$ s (our experiment), $f_0 = 4 \times 10^{12}$ s$^{-1}$, and $p \approx 10^{-4}$ (the temperature regime of our experiment and expected values for the energy barrier), so $n$, $np$, and $np(1-p)$ are all large compared to 1. Following the de Moivre-Laplace theorem [12], we perform a normal approximation and alter the relationship (14) to

$$n_{\mathrm{f}}(T) \sim \mathcal{N}(\mu, \sigma^2) \tag{16}$$

with the distribution parameters

$$\mu(T) = np = t_{\mathrm{f}} f_0 \exp\left(-\frac{E_{\mathrm{m}}}{k_{\mathrm{B}}T}\right), \tag{17}$$

$$\sigma(T) = \sqrt{np(1-p)} = \sqrt{t_\mathrm{f} f_0 e^{-\frac{E_\mathrm{m}}{k_\mathrm{B}T}} \left(1 - e^{-\frac{E_\mathrm{m}}{k_\mathrm{B}T}}\right)}, \tag{18}$$

and the probability density function (PDF)

$$p_\mathrm{f}\left(n_\mathrm{f}(T), T\right) = \left(2\pi\sigma^2\right)^{-1/2} \exp\left(-\frac{\left(n_\mathrm{f}(T) - \mu\right)^2}{2\sigma^2}\right). \tag{19}$$

Second, we describe vacancy healing: the adatom path length $n_\mathrm{h}^\mathrm{sv}$ is the number of single surface diffusion steps that an adatom needs to make until the immediate proximity of a single vacancy is reached. This is well-defined, since the migration path of a carbon adatom passes from one equivalent minimum-energy adsorption position above the bond center of two lattice atoms (changing their hybridization from $sp^2$-like to $sp^3$-like and establishing a carbon-carbon bridge) to the next [13]. $n_\mathrm{h}^\mathrm{sv}$ is a random variable that obeys the geometric distribution [14]

$$n_\mathrm{h}^\mathrm{sv} \sim \mathrm{Geo}\left(p'\right) \tag{20}$$

with the distribution parameter

$$p' = \frac{N_\mathrm{ad}}{N_\text{lattice-bonds}} =: \frac{2}{3} c_\mathrm{ad}, \tag{21}$$

where $c_\mathrm{ad}$ is the number of adatoms per lattice atom and the pre-factor $2/3$ accounts for number of lattice bonds per lattice atom. This was verified by Monte-Carlo simulations [15, 16] implemented in a small Python code. As an implication, adatom arrival is a Poisson process [17], which presumably also governs vacancy healing ($E_m \gg E_r$, see above). The continuous analogue of the geometric distribution is the exponential distribution [14, 18], so we replace relation (20) by

$$n_\mathrm{h}^\mathrm{sv} \sim \mathrm{Exp}\left(\nu^\mathrm{sv}\right) \tag{22}$$

with the distribution parameter (see Ref. [19])

$$\nu^\mathrm{sv} = -\log\left(1 - p'\right) = -\log\left(1 - \frac{2}{3} c_\mathrm{ad}\right), \tag{23}$$

and the PDF

$$p_\mathrm{h}^\mathrm{sv}\left(n_\mathrm{h}^\mathrm{sv}\right) = \nu^\mathrm{sv} e^{-n_\mathrm{h}^\mathrm{sv}\nu^\mathrm{sv}} = -\log\left(1 - p'\right) e^{n_\mathrm{h}^\mathrm{sv}\log(1-p')}. \tag{24}$$

The superscript sv denotes that we consider here the case of one missing atom, i.e., a single vacancy. The random variable relevant for the probability term $P_\mathrm{h}^\mathrm{sv}(T)$ is the quotient

$$Q^\mathrm{sv}(T) = n_\mathrm{f}(T)/n_\mathrm{h}^\mathrm{sv}. \tag{25}$$

Strictly speaking, we are interested in the complementary cumulative distribution function (CCDF) of the ratio distribution of equations (16) and (22). $n_\mathrm{f}(T)$ and $n_\mathrm{h}^\mathrm{sv}$ are independent and, thus, the PDF of $Q^\mathrm{sv}(T)$ is given by [20]

$$p_{Q^\mathrm{sv}}(q, T) = \int_{-\infty}^{\infty} p_\mathrm{f}\,(tq, T)\, p_\mathrm{h}^\mathrm{sv}\,(t)\,|t|\,\mathrm{d}t. \tag{26}$$

The cumulative distribution function (CDF) is now

$$P_{Q^\mathrm{sv}}(q, T) = \int_{-\infty}^{q} p_{Q^\mathrm{sv}}(q', T)\,\mathrm{d}q' \tag{27}$$

and the healing probability is given by the tail distribution

$$P_\mathrm{h}^\mathrm{sv}(T) = 1 - P_{Q^\mathrm{sv}}(1, T) = \int_{1}^{\infty} p_{Q^\mathrm{sv}}(q, T)\,\mathrm{d}q. \tag{28}$$

Last, we incorporate multi-atom vacancies into the model. This can formally be done by multiplying the denominator $n_\mathrm{h}^\mathrm{sv}$ in equation (25) by the average vacancy size $N_\mathrm{v}$,

$$Q(T) = \frac{Q^\mathrm{sv}(T)}{N_\mathrm{v}} = \frac{n_\mathrm{f}(T)}{N_\mathrm{v}\, n_\mathrm{h}} \tag{29}$$

This correction accordingly changes the distribution parameter in equation (23) to

$$\nu = \frac{\nu^\mathrm{sv}}{N_\mathrm{v}} = -\frac{1}{N_\mathrm{v}} \log\left(1 - \frac{2}{3} c_\mathrm{ad}\right), \tag{30}$$

which further propagates through equations (24)–(27) and yields the healing probability

$$P_\mathrm{h}(T) = \int_{1}^{\infty} p_Q(q, T)\,\mathrm{d}q = \int_{1}^{\infty} p_\mathrm{f}(tq, T) p_\mathrm{h}(t) |t|\,\mathrm{d}t. \tag{31}$$

Equation (31) was numerically solved, giving values slightly lower than 1. This shows that while there is a finite probability that a vacancy is not healed (and, thus, can be observed), this is no lower than 99.9 %, resulting in negligible predicted cross section values at temperatures above about 500 K. To recap, the exact form of our extended model, also see equation (4) of the main article, denotes

$$k_\mathrm{ko}^\mathrm{obs}(T) = k_\mathrm{ko}^\mathrm{theor}(T) - k_\mathrm{h}(T) = k_\mathrm{ko}^\mathrm{theor}(T)\,(1 - P_\mathrm{h}(T))\,. \tag{32}$$

In equations (7) and (8) of the main article, we describe an approximation of the healing probability of equation (31). The approximation is valid when the standard deviation of the number of steps taken (equation (18)) is much smaller than the distribution parameter of equation (23), i.e., $\sigma(T) \ll 1/\nu^\mathrm{sv}$, which is true for all reasonable experimental temperatures.

Furthermore, equation (8) of the main article can be simplified by using its first-order Taylor approximation, which leads to

$$k_{\mathrm{ko}}^{\mathrm{obs}}(T) \approx k_{\mathrm{ko}}^{\mathrm{theor}}(T) \max\left(0, 1 - \frac{2}{3N_{\mathrm{v}}} c_{\mathrm{ad}}(T) t_{\mathrm{f}} f_0 \exp\left(\frac{-E_{\mathrm{m}}}{k_{\mathrm{B}}T}\right)\right). \tag{33}$$

Thus, equation (33) describes the probability of vacancy healing within one frame time before knock-on damage can be observed. Numerical evaluation of this simplified model, according to equation (33), also yields $k_{\mathrm{ko}}^{\mathrm{obs}}(T) = 0$ for $T \geq 500$ K. As explained in the main article, this discrepancy is resolved by taking into account the shape of the electron probe.

A Supplementary data item (Jupyter notebook) contains the code used to simulate our extended model.

### 3. *Adatom concentration and temperature-dependence*

It should be noted that the adatom concentration can alternatively be expressed by areal concentrations, i.e. $c_{\mathrm{ad}} = \frac{c_{\mathrm{ad}}^{\mathrm{A}}}{\rho_A} = \frac{c_{\mathrm{ad}}^{\mathrm{A}} A_{\mathrm{UC}}}{2}$, where $A_{\mathrm{UC}} = \frac{a^2\sqrt{3}}{2} \approx 0.0524$ nm$^2$ is the area of a graphene unit cell ($a_{\mathrm{gra}} \approx 0.246$ nm). While this likely has some temperature-dependence, appropriate models and/or measurements are either lacking or describe incomparable systems [21], and thus this is neglected in our treatment. Future studies on this could be based upon former investigations by Hirsch et al. [21], He et al. [22], and related articles.

### D. Probe-shape measurement

We estimate the electron probe shape by matching the intensity of experimentally recorded images to a model image. Our approach is similar but not identical to a recently published method [23]. We model the image intensity as a superposition of rotationally symmetric probes $f$, placed at each atomic position with an additive background intensity $b$, giving

$$I_{model} = \sum_i f(\boldsymbol{x}_i) + b, \tag{34}$$

where $\boldsymbol{x}_\mathrm{i} = (x_\mathrm{i}, y_\mathrm{i})$ is the position of the $i^{\mathrm{th}}$ atom. This is a good approximation for 2D materials [24]. We find the atomic positions, $x_i$, using a machine-learning model published in a recent study [25].

The radially symmetric probe function, $f$, is modelled as a superposition of Gaussians

$$f(\boldsymbol{x}_i) = \sum_j a_j \exp(-\boldsymbol{x}_i^2/c_j), \tag{35}$$

where the set of parameters $\boldsymbol{a} = \{a_1, a_2, \ldots, a_N\}$ and $\boldsymbol{c} = \{c_1, c_2, \ldots, c_N\}$, are determined from the fitting procedure. We found that a superposition of four Gaussian components was sufficient.

The model image intensity is optimized by minimizing its difference to the experimental image intensity over the fitting parameters by using gradient descent:

$$\min_{\boldsymbol{a},\boldsymbol{c},b} \quad \sum (I_{model}(\boldsymbol{a}, \boldsymbol{c}, b) - I_{experiment})^2, \tag{36}$$

where we sum over the pixels of the image. The algorithm is implemented using the PyTorch library [26], whose automatic differentiation module is used to calculate gradients and the built-in stochastic gradient descent optimizer is used to update the solution. We start the optimization from multiple initial starting points to avoid only finding a poor local minimum, and run it until convergence.

We note that this method works best when it is used to model images with defects. When applied to images of an ideal lattice, we find that multiple different solutions for the probe can model very similar images, and hence the optimal image model might not result from the true probe shape.

### E. Experimental data

#### 1. *Measured knock-on damage cross sections*

Experimental image acquisition parameters and knock-on damage cross section values are listed in Tables I and II.

#### 2. *Beam-current calibration*

To estimate the beam current for each experimental data series, we used a separate calibration measurement where it was measured as a function of the virtual objective aperture (VOA) current, which is automatically written into the image metadata, on a regular basis (see Suppl. Fig. 5). For any given knock-on measurement, we acquired a current calibration within a time span of ±2 weeks. Note that the calibration recorded on June 30th, 2021, differed significantly from the rest, and thus a set of corresponding data ($T$ = 318 K) was omitted from the analyses.

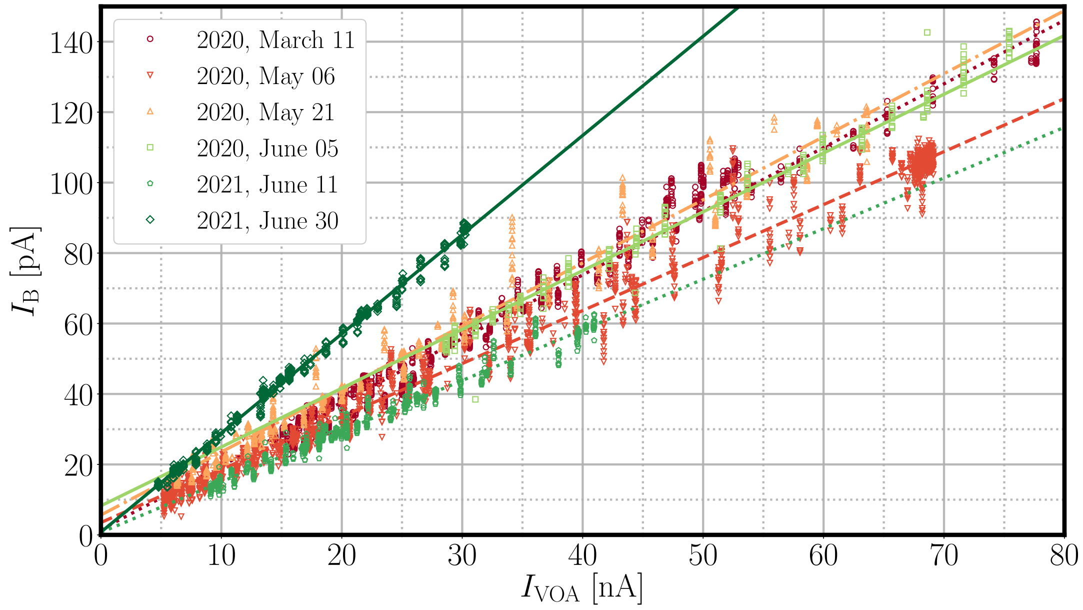


Supplemental Figure 5. Beam current $I_B$ as a function of virtual objective aperture (VOA) current $I_{VOA}$ at different points in time during the experimental schedule.

Table I. Experimental parameters and calculated values for all individually acquired image series. $T$ is the temperature, $N_{\mathrm{xy}}$ the number of pixels, $t_d$ the dwell time, $t_f$ the frame time, $A_{\mathrm{FOV}}$ the field of view, $\overline{I_{\mathrm{b}}}$ the mean beam current, $N_{\mathrm{ko}}^{\mathrm{obs}}$ the observed number of knock-on damage events, $\sigma^{\mathrm{obs}}$ the observed cross section, and $\sigma^{\mathrm{theor}}$ the theoretical cross section.

| $T$ [K] | $N_{\mathrm{xy}}$ | $t_d$ [$\mu$s] | $t_f$ [ms] | $A_{\mathrm{FOV}}$ [nm$^2$] | $\overline{I_b}$ [pA] | $N_{\mathrm{ko}}^{\mathrm{obs}}$ | $\sigma_{\mathrm{ko}}^{\mathrm{obs}}$ [mb] | $\sigma_{\mathrm{ko}}^{\mathrm{theor}}$ [mb] |
|---|---|---|---|---|---|---|---|---|
| 300 | $256^2$ | 8 | 524 | 1 | 115.8 | 67 | 13.6 ± 0.5 | 10.7 |
| | $512^2$ | 4 | 1049 | 1 | 106.8 | 66 | 10.4 ± 0.7 | |
| | $512^2$ | 4 | 1049 | 4 | 130.5 | 63 | 9.9 ± 0.5 | |
| 333 | $256^2$ | 8 | 524 | 1 | 125.9 | 57 | 11.9 ± 0.3 | 12.9 |
| | $256^2$ | 16 | 1049 | 1 | 118.2 | 51 | 9.0 ± 0.9 | |
| 373 | $256^2$ | 8 | 524 | 1 | 137.5 | 66 | 7.7 ± 0.3 | 16.0 |
| | $256^2$ | 16 | 1049 | 1 | 116.0 | 38 | 9.3 ± 0.6 | |
| | $256^2$ | 16 | 1049 | 4 | 124.0 | 75 | 8.8 ± 0.2 | |
| 473 | $256^2$ | 8 | 524 | 1 | 109.8 | 44 | 2.7 ± 0.2 | 26.5 |
| | $256^2$ | 16 | 1049 | 1 | 99.9 | 42 | 2.9 ± 0.1 | |
| 573 | $256^2$ | 8 | 524 | 1 | 119.5 | 76 | 7.3 ± 0.3 | 41.1 |
| | $256^2$ | 16 | 1049 | 1 | 129.7 | 56 | 4.3 ± 0.1 | |
| 673 | $128^2$ | 16 | 262 | 1 | 96.6 | 41 | 1.7 ± 0.1 | 59.9 |
| | $256^2$ | 8 | 524 | 1 | 97.0 | 56 | 3.1 ± 0.1 | |
| | $512^2$ | 2 | 524 | 1 | 110.7 | 41 | 2.3 ± 0.1 | |
| 873 | $256^2$ | 4 | 262 | 1 | 105.4 | 49 | 1.6 ± 0.1 | 108.7 |
| | $256^2$ | 8 | 524 | 1 | 88.5 | 43 | 6.5 ± 0.2 | |
| | $512^2$ | 2 | 524 | 1 | 130.4 | 48 | 4.5 ± 0.2 | |
| | $512^2$ | 8 | 2097 | 1 | 122.8 | 43 | 3.3 ± 0.1 | |
| 1073 | $256^2$ | 8 | 524 | 1 | 117.1 | 52 | 2.5 ± 0.3 | 169.8 |

Table II. Experimental parameters and calculated values for the image series merged w.r.t. temperature $T$. $\overline{I_{\mathrm{b}}}$ is the mean beam current, $N_{\mathrm{ko}}^{\mathrm{obs}}$ the observed number of knock-on damage events, $\sigma_{\mathrm{ko}}^{\mathrm{obs}}$ the observed cross section, and $\sigma_{\mathrm{ko}}^{\mathrm{theor}}$ the theoretical cross section.

| $T$ [K] | $\overline{I_b}$ [pA] | $N_{\mathrm{ko}}^{\mathrm{obs}}$ | $\sigma^{\mathrm{obs}}$ [mb] | $\sigma^{\mathrm{theor}}$ [mb] |
|---|---|---|---|---|
| 300 | 117.7 | 196 | $11.3 \pm 0.8$ | 10.7 |
| 333 | 125.6 | 108 | $10.6 \pm 1.3$ | 12.9 |
| 373 | 125.8 | 179 | $9.7 \pm 0.9$ | 16.0 |
| 473 | 104.8 | 86 | $2.8 \pm 0.3$ | 26.5 |
| 573 | 124.6 | 132 | $6.0 \pm 0.6$ | 41.1 |
| 673 | 101.4 | 138 | $2.5 \pm 0.2$ | 59.9 |
| 873 | 111.8 | 183 | $3.9 \pm 0.4$ | 108.7 |
| 1073 | 117.1 | 52 | $3.6 \pm 0.8$ | 169.8 |

### F. Uncertainty estimation

#### 1. Beam current

The beam current $I_\mathrm{B}$ was approximated based on the current $I_\mathrm{VOA}$ measured at the VOA by using a linear model function

$$I_\mathrm{B}\left(I_\mathrm{VOA}, a_1, a_2\right) = a_1\, I_\mathrm{VOA} + a_2, \tag{37}$$

whereby the parameters $a_i$ were obtained from a least-squares fit using data from a separate measurement in which, without a sample being present in the column, $I_\mathrm{VOA}$ and $I_\mathrm{B}$ were simultaneously recorded. Taking into account the correlation of $a_1$ and $a_2$, the used propagation of error formula for $I_\mathrm{B}$ is

$$\Delta I_\mathrm{B} = \sqrt{\underbrace{\left(\frac{\partial I_\mathrm{B}}{\partial a_1}\Delta a_1\right)^2 + \left(\frac{\partial I_\mathrm{B}}{\partial a_2}\Delta a_2\right)^2 + 2\frac{\partial I_\mathrm{B}}{\partial a_1}\frac{\partial I_\mathrm{B}}{\partial a_2}\, I_\mathrm{cov}\left(a_1, a_2\right)}_{=\mathrm{grad}_\mathbf{a}^\mathrm{T} I_\mathrm{B}\cdot \mathbf{V_a}\cdot \mathrm{grad}_\mathbf{a} I_\mathrm{B}} + \left(\underbrace{\frac{\partial I_\mathrm{B}}{\partial I_\mathrm{VOA}}}_{=a_1}\Delta I_\mathrm{VOA}\right)^2}\,, \tag{38}$$

where $\mathbf{V_a}$ is the covariance matrix of $\mathbf{a} = (a_1, a_2)$, and $\mathrm{grad}_\mathbf{a}$ is defined as $\left(\frac{\partial}{\partial a_1}, \frac{\partial}{\partial a_2}\right)$.

#### 2. Electron count

The number of electrons was calculated using the relationship

$$N_{\mathrm{e}^-} = \frac{1}{e}\left(\left(\sum_j t_j I_{\mathrm{B},j}\right) + \frac{t_\star}{2} I_{\mathrm{B},\star}\right), \tag{39}$$

where we summed up all frames before the defect occurred and took into account half of the time corresponding to the last frame $\star$, in which the defect appeared. We neglect the uncertainties of all time values before this frame, but evaluate its uncertainty as $\Delta\left(\frac{t_\star}{2}\right) = \frac{t_\star}{2}$ for frame $\star$. The used propagation of error formula for $N_{\mathrm{e}^-}$ is given by

$$\Delta N_{\mathrm{e}^-} = \frac{1}{e}\sqrt{\left(\sum_j \left(t_j \Delta I_{\mathrm{B},j}\right)^2\right) + \left(\frac{t_\star}{2}\Delta I_{\mathrm{B},\star}\right)^2 + \left(I_{\mathrm{B},\star}\frac{t_\star}{2}\right)^2}\,. \tag{40}$$

### 3. *Experimental cross section*

The best estimator of the cross section is given by $\sigma = \frac{1}{\rho_A \lambda}$ and its uncertainty by the propagation of error formula

$$\Delta\sigma = \frac{1}{\rho_A}\sqrt{\left(-\frac{1}{\lambda^2}\Delta\lambda\right)^2} = \frac{\Delta\lambda}{\rho_A \lambda^2} = \sigma\frac{\Delta\lambda}{\lambda}. \tag{41}$$

Additionally, we used the min-max method for propagating the uncertainties of the electron counts to the cross section by performing the same fit three times: $\{N_{\mathrm{e}^-}^{(i)}\} \to \lambda$, $\{N_{\mathrm{e}^-}^{(i)} + \Delta N_{\mathrm{e}^-}^{(i)}\} \to \lambda_{\mathrm{max}}$, and $\{N_{\mathrm{e}^-}^{(i)} - \Delta N_{\mathrm{e}^-}^{(i)}\} \to \lambda_{\mathrm{min}}$, where $k$ is the index for the corresponding knock-on event. This yields

$$\sigma_{\mathrm{min/max}} = \frac{1}{\rho_A \lambda_{\mathrm{max/min}}}. \tag{42}$$

In each case, the larger uncertainty value (according to equation (41) or (42)) is given in tables and used in plots.

### 4. *Observed knock-on rate*

The observed knock-on rate is given simply by

$$k_{\mathrm{ko}}^{\mathrm{obs}} = \frac{N_{\mathrm{ko}}}{t_{\mathrm{tot}}}. \tag{43}$$

Its propagation of error formula is

$$\Delta k_{\mathrm{ko}}^{\mathrm{obs}} = k_{\mathrm{ko}}^{\mathrm{obs}}\frac{\Delta t_{\mathrm{tot}}}{t_{\mathrm{tot}}}, \tag{44}$$

whereby the uncertainty of $t_{\mathrm{tot}}$ is given by

$$\Delta t_{\mathrm{tot}} = \sqrt{\sum_i \left(\Delta t_{\mathrm{tot}}^{(i)}\right)^2}. \tag{45}$$

### 5. *Theoretical cross section*

In our theoretical cross section model (Eq. (9)), the displacement threshold energy $T_{\mathrm{d}}$ and the variance of the normally distributed out-of-plane velocity of the lattice atoms with root-mean-square velocity $v_{\mathrm{rms}}(T) := (\overline{v^2})^{1/2} = (\int p(v,T)v^2\, dv)^{1/2}$ obtained from the phonon DOS model, were treated as variable parameters in order to fit the model curve to our experimental data points for room temperature at different voltages.

For the uncertainty of the cross section, we neglect the uncertainty of the acceleration voltage and use the propagation of error formula (omitting the label 'ko'), yielding

$$\Delta\sigma_{T_\mathrm{d},v_\mathrm{rms}} = \sqrt{\left(\frac{\partial\sigma_{T_\mathrm{d},v_\mathrm{rms}}}{\partial T_\mathrm{d}}\Delta T_\mathrm{d}\right)^2 + \left(\frac{\partial\sigma_{T_\mathrm{d},v_\mathrm{rms}}}{\partial v_\mathrm{rms}}\Delta v_\mathrm{rms}\right)^2 + 2\frac{\partial\sigma_{T_\mathrm{d},v_\mathrm{rms}}}{\partial T_\mathrm{d}}\frac{\partial\sigma_{T_\mathrm{d},v_\mathrm{rms}}}{\partial v_\mathrm{rms}} I_\mathrm{cov}\left(T_\mathrm{d}, v_\mathrm{rms}\right)}. \tag{46}$$

### 6. Predicted knock-on rate

The predicted knock-on rate was calculated using the relationship

$$k_\mathrm{ko}^\mathrm{theor} = \frac{\sum_i N_{\mathrm{e}^-}^{(i)}}{t_\mathrm{tot}}\,\rho_A\,\sigma^\mathrm{theor}. \tag{47}$$

Any uncertainty of the areal atomic density $\rho_A$ was neglected, and as for the uncertainty of $t_\mathrm{tot}$, this was taken into account in the uncertainty of the electron count $N_{\mathrm{e}^-}^{(i)}$. Thus, the propagation of error formula is

$$\Delta k_\mathrm{ko}^\mathrm{theor} = \frac{\rho_A}{t_\mathrm{tot}}\sqrt{\left(\sigma^\mathrm{theor}\right)^2\sum_i\left(\Delta N_{\mathrm{e}^-}^{(i)}\right)^2 + \left(\Delta\sigma^\mathrm{theor}\sum_i N_{\mathrm{e}^-}^{(i)}\right)^2}. \tag{48}$$

### 7. Migration energy barrier (Arrhenius formalism)

$E_\mathrm{m}$ and its uncertainty $\Delta E_\mathrm{m}$ were obtained from an orthogonal distance regression (ODR) fit using the linear model function

$$y\left(\frac{1}{T}\right) := \log\left(k_\mathrm{ko}^\mathrm{theor}(T) - k_\mathrm{ko}^\mathrm{obs}(T)\right) = \underbrace{-\frac{E_\mathrm{m}}{k_\mathrm{B}}}_{=:b_1}\frac{1}{T} + \underbrace{\log A}_{=:b_2}, \tag{49}$$

where the uncertainties

$$\frac{\Delta T}{T} = 0.05 \tag{50}$$

and

$$\Delta y = \frac{1}{|k_\mathrm{ko}^\mathrm{theor} - k_\mathrm{ko}^\mathrm{obs}|}\sqrt{\left(\Delta k_\mathrm{ko}^\mathrm{theor}\right)^2 + \left(\Delta k_\mathrm{ko}^\mathrm{obs}\right)^2} \tag{51}$$

were taken into account in the fitting procedure.

[1] T. Susi, J. C. Meyer, and J. Kotakoski, Nature Reviews Physics **1**, 397 (2019).

[2] F. Seitz and J. Koehler, *Solid state physics vol. 2* (Academic Press, New York, 1956).

[3] A. Zobelli, A. Gloter, C. P. Ewels, G. Seifert, and C. Colliex, Physical Review B **75**, 245402 (2007).

[4] T. Susi, C. Hofer, G. Argentero, G. T. Leuthner, T. J. Pennycook, C. Mangler, J. C. Meyer, and J. Kotakoski, Nature Communications **7**, 13040 (2016).

[5] N. F. Mott and N. H. D. Bohr, Proceedings of the Royal Society of London. Series A, Containing Papers of a Mathematical and Physical Character **124**, 425 (1929).

[6] N. F. Mott and R. H. Fowler, Proceedings of the Royal Society of London. Series A, Containing Papers of a Mathematical and Physical Character **135**, 429 (1932).

[7] W. A. McKinley and H. Feshbach, Physical Review **74**, 1759 (1948).

[8] A. R. Conn, N. I. Gould, and P. L. Toint, *Trust region methods* (SIAM, 2000).

[9] P. T. Boggs and J. E. Rogers, Contemporary Mathematics **112**, 183 (1990).

[10] K. J. Laidler, Journal of chemical Education **61**, 494 (1984), publisher: ACS Publications.

[11] J. Bernoulli, *Ars conjectandi, opus posthumum: accedit tractatus de seriebus infinitis, et epistola Gallice scripta de ludo pilæ reticularis* (Impensis Thurnisiorum Fratrum, 1713).

[12] A. De Moivre, *The doctrine of chances: A method of calculating the probabilities of events in play* (Routledge, 2020).

[13] P. O. Lehtinen, A. S. Foster, A. Ayuela, A. Krasheninnikov, K. Nordlund, and R. M. Nieminen, Physical Review Letters **91**, 017202 (2003).

[14] F. M. Dekking, C. Kraaikamp, H. P. Lopuhaä, and L. E. Meester, *A Modern Introduction to Probability and Statistics: Understanding Why and How* (Springer Science & Business Media, 2005).

[15] S. Ulam, R. D. Richtmyer, and J. von Neumann, Los Alamos National Laboratory **551**, 1 (1947).

[16] N. Metropolis and S. Ulam, Journal of the American statistical association **44**, 335 (1949).

[17] J. F. C. Kingman, *Poisson processes*, Vol. 3 (Clarendon Press, 1992).

[18] W. Von der Linden, V. Dose, and U. Von Toussaint, *Bayesian probability theory: applications in the physical sciences* (Cambridge University Press, 2014).

[19] J. Pitman, *Probability*, Springer Texts in Statistics (Springer-Verlag, New York, 1993).

[20] J. H. Curtiss, The Annals of Mathematical Statistics **12**, 409 (1941).

[21] P. Hirsch, M. Kässens, M. Püttmann, and L. Reimer, Scanning **16**, 101 (1994).

[22] K. He, A. W. Robertson, Y. Fan, C. S. Allen, Y.-C. Lin, K. Suenaga, A. I. Kirkland, and J. H. Warner, ACS Nano **9**, 4786 (2015).

[23] C. Hofer, V. Skákalová, J. Haas, X. Wang, K. Braun, R. S. Pennington, and J. C. Meyer, Ultramicroscopy **227**, 113292 (2021).

[24] E. J. Kirkland, *Advanced Computing in Electron Microscopy*, 2nd ed. (Springer US, 2010).

[25] A. Trentino, J. Madsen, A. Mittelberger, C. Mangler, T. Susi, K. Mustonen, and J. Kotakoski, Nano Letters **21**, 5179 (2021).

[26] A. Paszke, S. Gross, F. Massa, A. Lerer, J. Bradbury, G. Chanan, T. Killeen, Z. Lin, N. Gimelshein, L. Antiga, A. Desmaison, A. Kopf, E. Yang, Z. DeVito, M. Raison, A. Tejani, S. Chilamkurthy, B. Steiner, L. Fang, J. Bai, and S. Chintala, in *Advances in Neural Information Processing Systems 32*, edited by H. Wallach, H. Larochelle, A. Beygelzimer, F. d. Alché-Buc, E. Fox, and R. Garnett (Curran Associates, Inc., 2019) pp. 8024–8035.
